# Supplementary material for: High-fidelity two-qubit gates in silicon above one Kelvin
Source: arXiv:2007.09034 ancillary file (2020-07-17)
Supplement: Supplementary file 1 [file SupplementaryMaterial.pdf]

# Supplemental Material

## I. RECONSTRUCTION OF THE SPIN STATE PROBABILITIES

In order to readout the spin states we average all single-shot readout traces and subtract a reference sequence in which no gates are performed. The corresponding readout signal is therefore a current that is proportional to the probability of having a blocked state. In order to be able to reconstruct the four probability amplitudes $|A|^2, |B|^2, |C|^2, |D|^2$ of an arbitrary state $\psi = A\left|\uparrow\uparrow\right\rangle + B\left|\uparrow\downarrow\right\rangle + C\left|\downarrow\uparrow\right\rangle + D\left|\downarrow\downarrow\right\rangle$ it is necessary to know the current signal of the four spin states $\{\alpha \longrightarrow \left|\downarrow\uparrow\right\rangle, \beta \longrightarrow \left|\uparrow\uparrow\right\rangle, \gamma \longrightarrow \left|\downarrow\downarrow\right\rangle, \delta \longrightarrow \left|\uparrow\downarrow\right\rangle\}$. By initializing the $\left|\downarrow\uparrow\right\rangle$ state and then using the four frequencies $\mathrm{f}_1, \mathrm{f}_2, \mathrm{f}_3, \mathrm{f}_4$ we can reach all spin states and therefore measure the parameters $\alpha, \beta, \gamma, \delta$.

Once we measure the current signals for all spin states we need to gain information about the state $\psi$. We therefore apply the following sequences and measure the parameters $\phi_0, \phi_1, \phi_2, \phi_3$:

- Sequence: prepare state $\psi$ and then measure. We measure a current $\phi_0$ equal to:

$$\phi_0 = |A|^2\beta + |B|^2\delta + |C|^2\alpha + |D|^2\gamma \tag{1}$$

- Sequence: prepare state $\psi$, apply a $\pi$ pulse on f1, and then measure. We measure a current $\phi_1$ equal to:

$$\phi_1 = |C|^2\beta + |B|^2\delta + |A|^2\alpha + |D|^2\gamma \tag{2}$$

- Sequence: prepare state $\psi$, apply a $\pi$ pulse on f0, and then measure. We measure a current $\phi_2$ equal to:

$$\phi_2 = |A|^2\beta + |B|^2\delta + |D|^2\alpha + |C|^2\gamma \tag{3}$$

- Sequence: prepare state $\psi$, apply a $\pi$ pulse on f2, apply a $\pi$ pulse on f1, and then measure. We measure a current $\phi_3$ equal to:

$$\phi_3 = |C|^2\beta + |A|^2\delta + |B|^2\alpha + |D|^2\gamma \tag{4}$$

Therefore we have the following system of equations, that we want to solve for the probabilities $|A|^2, |B|^2, |C|^2, |D|^2$:

$$\begin{bmatrix} \beta & \delta & \alpha & \gamma \\ \alpha & \delta & \beta & \gamma \\ \beta & \delta & \gamma & \alpha \\ \delta & \alpha & \beta & \gamma \end{bmatrix} \cdot \begin{bmatrix} |A|^2 \\ |B|^2 \\ |C|^2 \\ |D|^2 \end{bmatrix} = \begin{bmatrix} \phi_0 \\ \phi_1 \\ \phi_2 \\ \phi_3 \end{bmatrix} \tag{5}$$

We solve the system by inverting the matrix:

$$\begin{bmatrix} |A|^2 \\ |B|^2 \\ |C|^2 \\ |D|^2 \end{bmatrix} = \begin{bmatrix} \beta & \delta & \alpha & \gamma \\ \alpha & \delta & \beta & \gamma \\ \beta & \delta & \gamma & \alpha \\ \delta & \alpha & \beta & \gamma \end{bmatrix}^{-1} \cdot \begin{bmatrix} \phi_0 \\ \phi_1 \\ \phi_2 \\ \phi_3 \end{bmatrix} \tag{6}$$

Finally the resulting amplitudes are normalized. The extracted probabilities correspond to the diagonal parts of the density matrix $\rho$ which may violate $\sum_i \rho_{ii} = 1$ due to measurement and gate errors. In order to ensure the physicality of our results we perform a maximum-likelihood estimation [1] using the diagonal elements of the density matrix.

## II. EXCHANGE SPECTRUM

Supplemental Fig. 1a shows the exchange spectrum as a function of detuning. When $J < 10\,\mathrm{MHz}$ we measure the exchange interaction by mapping $f_1, f_2, f_3, f_4$ as a function of the detuning energy $\epsilon$ and then extract $J$ as the difference between $f_1$ and $f_2$, and $f_3$ and $f_4$ respectively. When $J > 10\,\mathrm{MHz}$ we extract the exchange from the frequency of the SWAP oscillations given by $f_{\mathrm{SWAP}} = \sqrt{J^2 + \Delta E_{\mathrm{z}}^2}$.

The best agreement to our data set is obtained by fitting with an exponential dependence [2, 3] $J(\epsilon) = \exp(2\alpha(\epsilon - V_0))$ and constant $\Delta E_{\mathrm{z}}(\epsilon) = \Delta E_{\mathrm{z}}$ with parameters $\alpha = -0.022\,\ln(\mathrm{MHz})/\mathrm{mV}$, $V_0 = 120\,\mathrm{mV}$, and $\Delta E_{\mathrm{z}} = 11\,\mathrm{MHz}$.

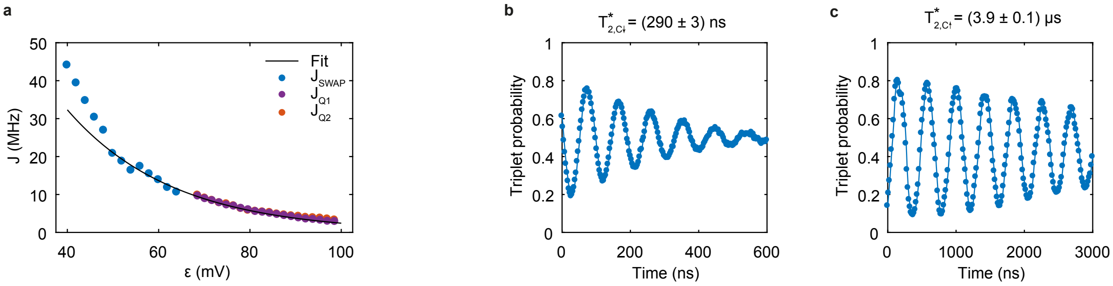


Figure 1. **Exchange interaction a** Exchange energy as a function of detuning energy. The data points $J_{\mathrm{SWAP}}$ have been extracted from the frequency of SWAP oscillations, $J_{\mathrm{Q1}}$ and $J_{\mathrm{Q2}}$ are obtained from the energy difference between $f_1$ and $f_2$, and $f_3$ and $f_4$ respectively. The fit (solid black line) is used for the results in the main text. We observe frequency jumps in the first five points of the data set, and these are therefore neglected in the fitting. **b-c** Simulated data for the sequence used in Fig. 2a and 2b of the main text.

## III. TWO-QUBIT GATE SIMULATIONS

### A. Physical model

For all the two-qubit gates we obtain the fidelities by numerically solving the time-dependent Schrodinger equation $i\hbar\dot{\Psi}(t) = H(t)\Psi(t)$ using a step size $t = 50\,\mathrm{ps}$. We have confirmed that a faster sampling rate does not change the simulation results. In order to resemble real setups and to avoid sampling problems we filter all time-dependent signals using a high-pass filter with a cut-off frequency of 300 MHz. All simulations are performed using the Heisenberg Hamiltonian

$$H(t) = \Delta E_{\mathrm{z}}(\epsilon)(S_{\mathrm{z},1} - S_{\mathrm{z},2})/2 + J(\epsilon)(\boldsymbol{S}_1 \cdot \boldsymbol{S}_2 - 1/4), \quad (7)$$

where $\boldsymbol{S}_i = (S_{\mathrm{x,i}}, S_{\mathrm{y,i}}, S_{\mathrm{z,i}})$ is the spin operator of the electron in quantum dot $i$. The parameters $\Delta E_{\mathrm{z}}(\epsilon)$ and $J(\epsilon)$ are the qubit frequency difference and the exchange interaction which both depend on the detuning $\epsilon$.

To include the effect of decoherence we add stochastic fluctuations of the detuning, $\epsilon \to \epsilon + \delta\epsilon(t)$ to each run of the time evolution and average the resulting density matrix. To emulate the effect of $1/f$ charge noise we generate time-dependent fluctuations $\delta\epsilon(t)$ following a $S(\omega) = A_\epsilon/f$ spectral density using the method described in Ref. [4, 5]. The amplitude of the noise $A_\epsilon$ is set such that it reproduces the decay time of the exchange oscillations measured experimentally. Using the same value of noise we then simulate the Ramsey sequences of Fig. 2a and 2b of the main text and we show the results in Fig. 1b and 1c. The decay times that we extract are in agreement with the measured decays $T^*_{2,\mathrm{C}\downarrow} = (397 \pm 24)$ ns and $T^*_{2,\mathrm{C}\uparrow} = (3.9 \pm 0.6)$ µs, where $C$ refers to the control qubit.

For benchmarking the performance of the simulated gate operations we use the average gate fidelity from QuTiP [6].

### B. Adiabatic and diabatic CPHASE gates

Using the Hamiltonian in Eq. 7 it is possible to implement a controlled-phase (CPHASE) gate. The conventional approach for the CPHASE implementation is to use a smooth exchange pulse such that the system undergoes a adiabatic time evolution and it accumulates a phase difference between the even $\{|\uparrow\uparrow\rangle, |\downarrow\downarrow\rangle\}$ and odd parity subspace $\{|\uparrow\downarrow\rangle, |\downarrow\uparrow\rangle\}$. The adiabatic time evolution of the system described by the Hamiltonian in Eq. 7 is the unitary

$$U_{\mathrm{ad}} = e^{-i\Phi(S_{z,1}S_{z,2}-1/4)} \times e^{-i(\theta_{\mathrm{ad}}-\theta_{\mathrm{res}})(S_{\mathrm{z},1}-S_{\mathrm{z},2})/2} \quad (8)$$

with the entangling phase $\Phi = \int_0^t (J(t') - J_{\mathrm{res}})dt'/\hbar$ and the single-qubit phases $\theta_{\mathrm{ad}} = \int_0^t \sqrt{\Delta E_z^2 + J^2(t')}dt'/\hbar$ and $\theta_{\mathrm{res}} = \sqrt{\Delta E_z^2 + J_{\mathrm{res}}^2}\,t/\hbar$. Here we explicitly took into consideration that $J(t=0) = J_{\mathrm{res}}$. An adiabatic CPHASE gate is then obtained for $\Phi = (2n+1)\pi$ with $n$ being an integer number. Virtual single-qubit z-gates are then applied to compensate for the single-qubit phase evolution $\theta_{\mathrm{ad}}$. Non-adiabatic (diabatic) errors due to a violation of the adiabatic condition enter via spin-flip terms $S_{\mathrm{x},1}S_{\mathrm{x},2} + S_{\mathrm{y},1}S_{\mathrm{y},2}$ and $S_{\mathrm{x},1}S_{\mathrm{y},2} - S_{\mathrm{y},1}S_{\mathrm{z},2}$ and give rise to SWAP oscillations. They can be mitigated using a decoupling scheme [7] or sufficiently long ramp times (see Fig. 3a in the main text).

Faster CPHASE gates can be realized using diabatic pulses where we synchronize the SWAP oscillation with the CPHASE evolution [8]. The diabatic time evolution of a system described by Eq. 7 is given by:

$$U_{\mathrm{dia}} = e^{-i\Phi(S_{z,1}S_{z,2}-1/4)} \times e^{i\theta_{\mathrm{res}}(S_{z,1}-S_{z,2})/2}\left(\cos(\theta_{\mathrm{dia}}) - i\sin(\theta_{\mathrm{dia}})\frac{\boldsymbol{r}\cdot\boldsymbol{\sigma}}{|\boldsymbol{r}|}\right), \tag{9}$$

where $\boldsymbol{r} = (\Delta E_{\mathrm{z}}\cdot J - \Delta E_{\mathrm{z}}\cdot J_{\mathrm{res}}, 0, \Delta E_{\mathrm{z}}^2 + J\cdot J_{\mathrm{res}})$ describes the tilted SWAP rotation, $\theta_{\mathrm{dia}} = \sqrt{\Delta E_{\mathrm{z}}^2 + J^2}t/\hbar$ the angle of the rotation, and $\boldsymbol{\sigma} = (\hat{X}, \hat{Y}, \hat{Z})$ is the vector consisting of Pauli matrices in the odd parity space

$$\hat{X} = |\uparrow\downarrow\rangle\langle\downarrow\uparrow| + |\downarrow\uparrow\rangle\langle\uparrow\downarrow| \tag{10}$$

$$\hat{Y} = -i\,|\uparrow\downarrow\rangle\langle\downarrow\uparrow| + i\,|\downarrow\uparrow\rangle\langle\uparrow\downarrow| \tag{11}$$

$$\hat{Z} = |\uparrow\downarrow\rangle\langle\uparrow\downarrow| - |\downarrow\uparrow\rangle\langle\downarrow\uparrow| = S_{\mathrm{z},1} - S_{\mathrm{z},2}. \tag{12}$$

Note, that we again took into consideration that $J(t=0) = J_{\mathrm{res}}$ and assumed a piece-wise constant exchange pulse of the form

$$J(t) = \begin{cases} J & \text{if } t > 0 \text{ and } t \leq t_{\mathrm{end}} \\ J_{\mathrm{res}} & \text{else} \end{cases}. \tag{13}$$

A diabatic CPHASE gate is then given for $\Phi = (2n+1)\pi$ and $\theta_{\mathrm{dia}} = m\pi$ with $m, n$ being integers. A generic solution for $J$, which satisfies both constraints, is given by

$$J = \frac{\sqrt{-(2n+1)^2\left(\Delta E_{\mathrm{z}}^2\left((2n+1)^2 - 4m^2\right) - 4J_{\mathrm{res}}^2 m^2\right)} + 4J_{\mathrm{res}}m^2}{4m^2 - (2n+1)^2}. \tag{14}$$

The formula in the main text is obtained for $n = 0$ and $m = 1$, while the results in Ref. [8] are obtained for $J_{\mathrm{res}} = 0$.

## C. SWAP gate

For $\Delta E_{\mathrm{z}} = J_{\mathrm{res}} = 0$ the time-evolution of Eq. 9 gives rise to oscillations between the $|\uparrow\downarrow\rangle$ and $|\downarrow\uparrow\rangle$ states which can be used to implement the classical SWAP and maximally entangling $\sqrt{\mathrm{SWAP}}$ gate [9]. This is not the case for a finite $\Delta E_{\mathrm{z}} \neq 0$ and $J_{\mathrm{res}} > 0$ and the maximum flip probability is limited to

$$P_{\mathrm{flip}} = |\langle\uparrow\downarrow| U_{\mathrm{dia}} |\downarrow\uparrow\rangle|^2 = \frac{\Delta E_{\mathrm{z}}^2 (J - J_{\mathrm{res}})^2}{(\Delta E_{\mathrm{z}}^2 + J^2)(\Delta E_{\mathrm{z}}^2 + J_{\mathrm{res}})} \tag{15}$$

heavily reducing the maximum fidelity. When $J_{\mathrm{res}} = 3\,\mathrm{MHz}, \Delta E_{\mathrm{z}} = 11\,\mathrm{MHz}$ and $J = 27\,\mathrm{MHz}$ we obtain a maximum flip probability $P_{\mathrm{flip}} = 63\,\%$ which is a close match to the observed value in Figure 3c of the main text. From the formula above it is clear that a high-fidelity implementation of a SWAP gate with $J_{\mathrm{res}} = 3\,\mathrm{MHz}$ and $\Delta E_{\mathrm{z}} = 11\,\mathrm{MHz}$ would require an extremely large exchange interaction, usually not achieved in state-of-the-art experiments in silicon. Furthermore, it is also impossible to implement a high-fidelity entangling $\sqrt{\mathrm{SWAP}}$ in such a way due to the requirement $\sqrt{\mathrm{SWAP}}\sqrt{\mathrm{SWAP}} = \mathrm{SWAP}$.

In order to overcome these issues we decompose our desired SWAP rotation in the odd parity subspace in terms of tilted $\boldsymbol{r}$ rotations from the diabatic time evolution and $\boldsymbol{z}$ rotations from the adiabatic phase evolution. We then construct a composite pulse sequence by alternating diabatic and adiabatic pulses which yields our desired operation $U_{\mathrm{tot}}$

$$U_{\mathrm{tot}} = U_{\mathrm{dia}}(t_1, J_1)U_{\mathrm{ad}}(t_2, J_2)U_{\mathrm{dia}}(t_3, J_3)U_{\mathrm{ad}}(t_4, J_4)\cdots \tag{16}$$

Here, the tuple $(t_i, J_i)$ defines a diabatic or adiabatic pulse with time $t_i$ and exchange $J_i$. The total number of pulses for a SWAP are estimated to be $N = 2\left\lfloor \frac{90^\circ}{\beta} \right\rfloor$, where $\lfloor\cdot\rfloor$ is the floor function and $\beta$ denotes the angle between the vectors $\boldsymbol{r}$ and $\boldsymbol{z} = (0, 0, 1)$. Note, that the final $U_{\mathrm{ad}}$ operation only needs to correct single qubit phases which in our experiment can be done alternatively using virtual single qubit z-gates.

Enforcing the constraint $\Phi_{\mathrm{tot}} = \Phi_1 + \Phi_2 + \Phi_3 + \Phi_4 + \cdots = m\pi$, with integer $m$ and $\Phi_i$ being the entangling phase of the pulse $U_{\mathrm{dia,ad}}(t_i, J_i)$, ensures that the composite pulse yields a SWAP gate. Using instead $\Phi_{\mathrm{tot}} = \Phi_1 + \Phi_2 + \Phi_3 + \Phi_4 + \cdots = m\pi/2$ yields the universal $i$SWAP gate.

In our experiment we choose a minimal length symmetric composite pulse consisting of two identical diabatic pulses $U_{\rm dia}(t_1, J_1) = U_{\rm dia}(t_3, J_3) = U_{\rm r}(t_{\rm SWAP}, J)$ and an adiabatic pulse $U_{\rm ad}(t_2, J_2) = U_{\rm z}(t_{\rm corr}, J_{\rm corr})$ in between, $U_{\rm r}U_{\rm r}U_{\rm r} = \hat{X}$. The first diabatic pulse executes half of the desired SWAP rotation, the adiabatic pulse realizes a rotation in the $X-Y$-plane, and the second diabatic pulses finalizes the SWAP rotation. The pulse times are given by the conditions

$$t_{\rm SWAP} = \frac{2\hbar \sin^{-1}\left(\frac{1}{\sqrt{2P_{\rm flip}}}\right)}{\sqrt{\Delta E_{\rm z}^2 + J^2}}, \tag{17}$$

$$\int_{t_{\rm SWAP}}^{t_{\rm SWAP}+t_{\rm corr}} \sqrt{\Delta E_{\rm z}^2 + J_{\rm corr}^2(t')}dt' = 2\hbar \cos^{-1}\left(-\frac{\sqrt{(J^2-\Delta E_{\rm z}^2)(\Delta E_{\rm z}^2 - J_{\rm res}^2) - 4\Delta E_{\rm z}^2\, J\, J_{\rm res}}}{\Delta E_{\rm z}(J - J_{\rm res})}\right) \tag{18}$$

and the condition for the entangling phase $\Phi_{\rm tot}$ reads

$$2\,\hbar J\, t_{\rm SWAP} + \hbar \int_{t_{\rm SWAP}}^{t_{\rm SWAP}+t_{\rm corr}} J_{\rm corr}(t')dt' = m\pi. \tag{19}$$

Using a numerical search we find that the pulse sequence

$$J_{\rm corr}(t) = \begin{cases} 2.37\,{\rm MHz} \times \frac{t}{t_{\rm ramp}} & \text{if } t > 0 \text{ and } t \le t_{\rm ramp} \\ 2.37\,{\rm MHz} & \text{if } t > t_{\rm ramp} \text{ and } t_{\rm SWAP} - t_{\rm ramp} \\ 2.37\,{\rm MHz} \times \frac{t - t_{\rm SWAP} + t_{\rm ramp}}{t_{\rm ramp}} & \text{if } t > t_{\rm SWAP} - t_{\rm ramp} \text{ and } t \le t_{\rm SWAP} \\ 0 & \text{else} \end{cases} \tag{20}$$

allows to achieve gate fidelities $F > 99.9\,\%$.


[1] D. F. V. James, P. G. Kwiat, W. J. Munro, and A. G. White, Physical Review A **64**, 052312 (2001).
[2] O. E. Dial, M. D. Shulman, S. P. Harvey, H. Bluhm, V. Umansky, and A. Yacoby, Physical Review Letters **110**, 146804 (2013).
[3] P. Cerfontaine, T. Botzem, D. P. DiVincenzo, and H. Bluhm, Physical Review Letters **113**, 150501 (2014).
[4] J. V. Koski, A. J. Landig, M. Russ, J. C. Abadillo-Uriel, P. Scarlino, B. Kratochwil, C. Reichl, W. Wegscheider, G. Burkard, M. Friesen, S. N. Coppersmith, A. Wallraff, K. Ensslin, and T. Ihn, Nature Physics **16**, 642 (2020).
[5] Y.-C. Yang, S. N. Coppersmith, and M. Friesen, npj Quantum Information **5**, 1 (2019).
[6] J. Johansson, P. Nation, and F. Nori, Computer Physics Communications **184**, 1234 (2013).
[7] M. Russ, D. M. Zajac, A. J. Sigillito, F. Borjans, J. M. Taylor, J. R. Petta, and G. Burkard, Physical Review B **97**, 085421 (2018).
[8] G. Burkard, D. Loss, D. P. DiVincenzo, and J. A. Smolin, Physical Review B **60**, 11404 (1999).
[9] D. Loss and D. P. DiVincenzo, Physical Review A **57**, 120 (1998).
